# Supplementary material for: Stochastic Vision Transformers with Wasserstein Distance-Aware Attention
Source: arXiv:2311.18645 source file (2023-11-30)
Supplement: Supplementary file 1 [file 9_appendix.tex]

\section{Appendix}~\label{sec:appendix}
